# Supplementary material for: Mad Max: Affine Spline Insights into Deep Learning
Source: arXiv:1805.06576 source file (2018-11-11)
Supplement: Supplementary file 2 [file appendix_main.tex]

%%%%%%%% ICML 2018 EXAMPLE LATEX SUBMISSION FILE %%%%%%%%%%%%%%%%%

\documentclass{article}

\input{preamble}

% Recommended, but optional, packages for figures and better typesetting:
\usepackage{microtype}
\usepackage{graphicx}
\usepackage{subfigure}
\usepackage{booktabs} % for professional tables

% hyperref makes hyperlinks in the resulting PDF.
% If your build breaks (sometimes temporarily if a hyperlink spans a page)
% please comment out the following usepackage line and replace
% \usepackage{icml2018} with \usepackage[nohyperref]{icml2018} above.
\usepackage{hyperref}

% Attempt to make hyperref and algorithmic work together better:

% Use the following line for the initial blind version submitted for review:
\usepackage{icml2018}

% If accepted, instead use the following line for the camera-ready submission:
%\usepackage[accepted]{icml2018}

% The \icmltitle you define below is probably too long as a header.
% Therefore, a short form for the running title is supplied here:
\icmltitlerunning{A Spline Theory of Deep Networks}

\begin{document}

\twocolumn[
\icmltitle{A Spline Theory of Deep Networks}

% It is OKAY to include author information, even for blind
% submissions: the style file will automatically remove it for you
% unless you've provided the [accepted] option to the icml2018
% package.

% List of affiliations: The first argument should be a (short)
% identifier you will use later to specify author affiliations
% Academic affiliations should list Department, University, City, Region, Country
% Industry affiliations should list Company, City, Region, Country

% You can specify symbols, otherwise they are numbered in order.
% Ideally, you should not use this facility. Affiliations will be numbered
% in order of appearance and this is the preferred way.
\icmlsetsymbol{equal}{*}

\begin{icmlauthorlist}
\icmlauthor{Aeiau Zzzz}{equal,to}
\icmlauthor{Bauiu C.~Yyyy}{equal,to,goo}
\icmlauthor{Cieua Vvvvv}{goo}
\icmlauthor{Iaesut Saoeu}{ed}
\icmlauthor{Fiuea Rrrr}{to}
\icmlauthor{Tateu H.~Yasehe}{ed,to,goo}
\icmlauthor{Aaoeu Iasoh}{goo}
\icmlauthor{Buiui Eueu}{ed}
\icmlauthor{Aeuia Zzzz}{ed}
\icmlauthor{Bieea C.~Yyyy}{to,goo}
\icmlauthor{Teoau Xxxx}{ed}
\icmlauthor{Eee Pppp}{ed}
\end{icmlauthorlist}

\icmlaffiliation{to}{Department of Computation, University of Torontoland, Torontoland, Canada}
\icmlaffiliation{goo}{Googol ShallowMind, New London, Michigan, USA}
\icmlaffiliation{ed}{School of Computation, University of Edenborrow, Edenborrow, United Kingdom}

\icmlcorrespondingauthor{Cieua Vvvvv}{c.vvvvv@googol.com}
\icmlcorrespondingauthor{Eee Pppp}{ep@eden.co.uk}

% You may provide any keywords that you
% find helpful for describing your paper; these are used to populate
% the "keywords" metadata in the PDF but will not be shown in the document
\icmlkeywords{Deep learning, neural network, splines}

\vskip 0.3in
]

% this must go after the closing bracket ] following \twocolumn[ ...

% This command actually creates the footnote in the first column
% listing the affiliations and the copyright notice.
% The command takes one argument, which is text to display at the start of the footnote.
% The \icmlEqualContribution command is standard text for equal contribution.
% Remove it (just {}) if you do not need this facility.

%\printAffiliationsAndNotice{}  % leave blank if no need to mention equal contribution
\printAffiliationsAndNotice{\icmlEqualContribution} % otherwise use the standard text.

\appendix
\onecolumn

\begin{center}
\vspace{5mm}
{\LARGE SUPPLEMENTARY MATERIAL} %\\[5mm]
%{\Large A Spline Theory of Signal Processing}
\end{center}
We first present the topologies used in the experiments except for the Resnet4-4 being the standard wide resnet based topology with depth $4$ and width $4$.
We thus have for the smallCNN:
\begin{verbatim}
Conv2DLayer(layers[-1],32,3,pad='valid')
Pool2DLayer(layers[-1],2)
Conv2DLayer(layers[-1],64,3,pad='valid')
Pool2DLayer(layers[-1],2)
Conv2DLayer(layers[-1],128,1,pad='valid')
Pool2DLayer(layers[-1],2)
\end{verbatim}
and for the largeCNN:
\begin{verbatim}
Conv2DLayer(layers[-1],96,3,pad='same')
Conv2DLayer(layers[-1],96,3,pad='full')
Conv2DLayer(layers[-1],96,3,pad='full')
Pool2DLayer(layers[-1],2)
Conv2DLayer(layers[-1],192,3,pad='valid')
Conv2DLayer(layers[-1],192,3,pad='full')
Conv2DLayer(layers[-1],192,3,pad='valid')
Pool2DLayer(layers[-1],2)
Conv2DLayer(layers[-1],192,3,pad='valid')
Conv2DLayer(layers[-1],192,1)
Pool2DLayer(layers[-1],2)
\end{verbatim}
\newpage
\input{APPENDIX/notation}
\newpage
%\tableofcontents
\newpage
\input{APPENDIX/background}
\newpage
\input{APPENDIX/affine}%here are the explicit formula
\newpage
\input{APPENDIX/more_template}
\newpage
\input{APPENDIX/more_orthogonal}
\newpage
\input{APPENDIX/more_partitioning}

\bibliography{../ref}
\bibliographystyle{../icml2018}

\end{document}
