# Supplementary material for: Mad Max: Affine Spline Insights into Deep Learning
Source: arXiv:1805.06576 source file (2018-11-11)
Supplement: Supplementary file 3 [file more_orthogonal.tex]

\section{Additional Figures and Experiments with Orthogonal Templates}
\begin{figure}[H]
    \centering
    \includegraphics[width=.99\textwidth]{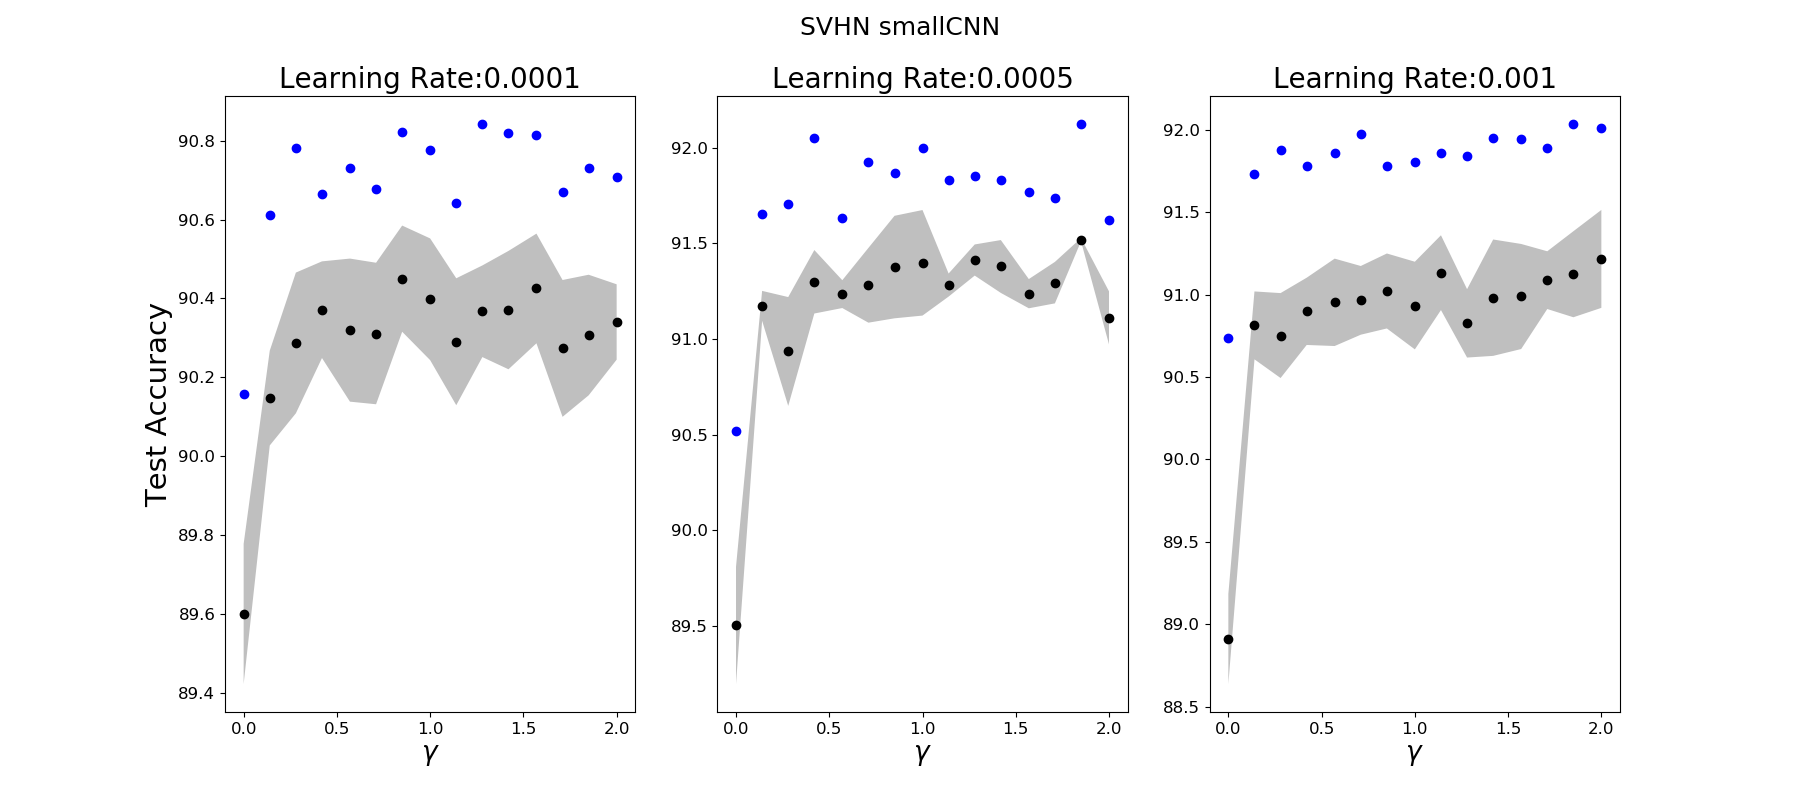}
    \end{figure}
    
\begin{figure}[H]
    \centering
    \includegraphics[width=.99\textwidth]{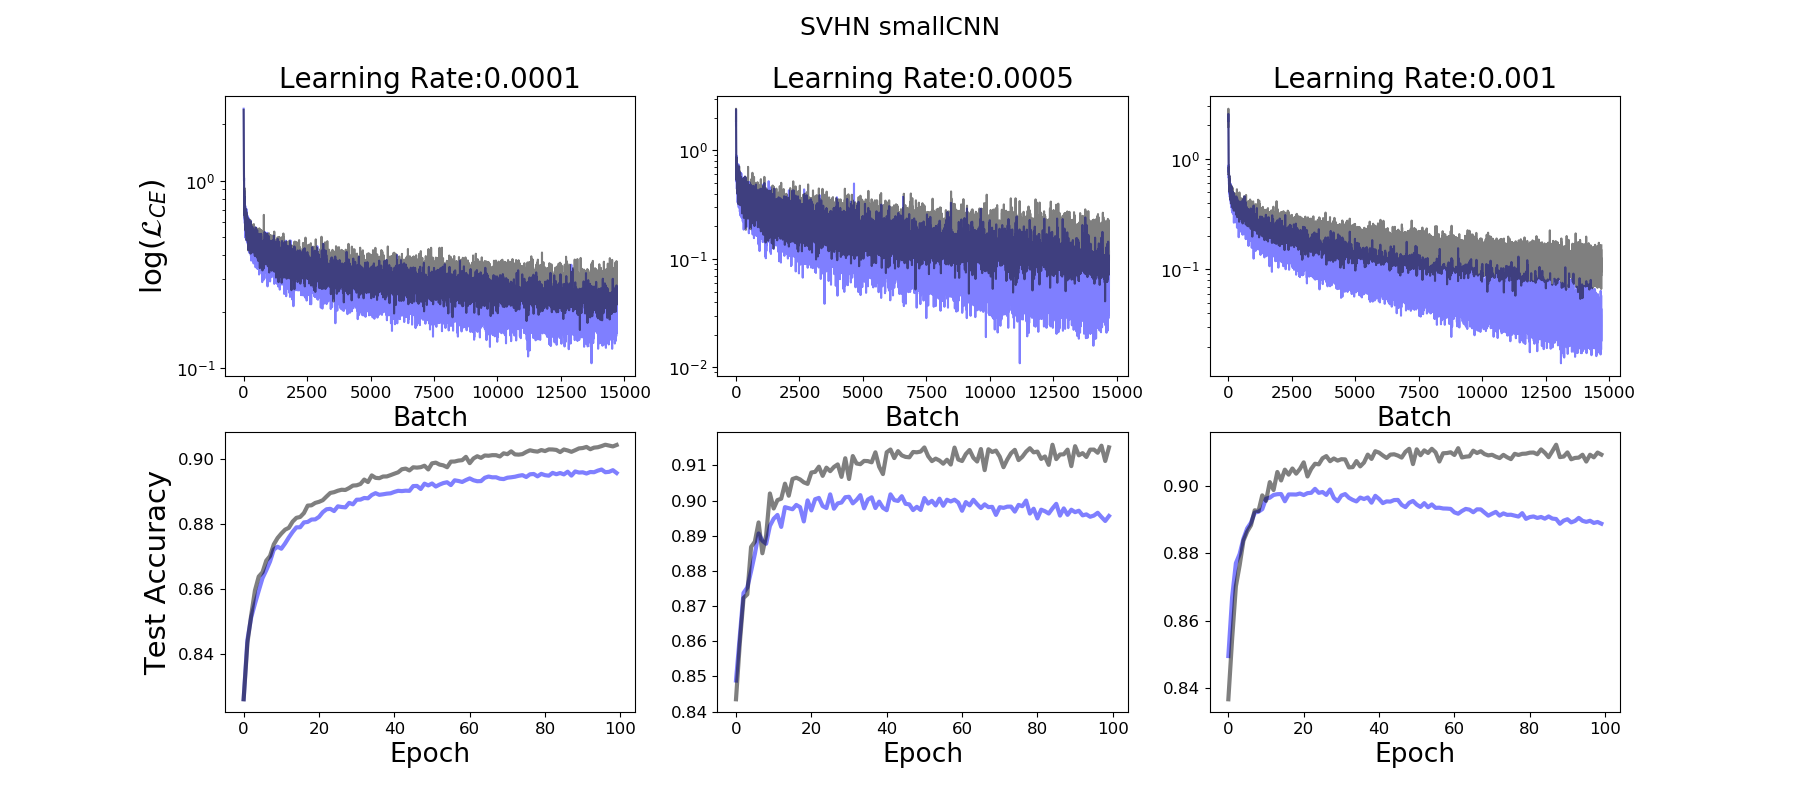}
    \end{figure}
    
    
\begin{figure}[H]
    \centering
    \includegraphics[width=.99\textwidth]{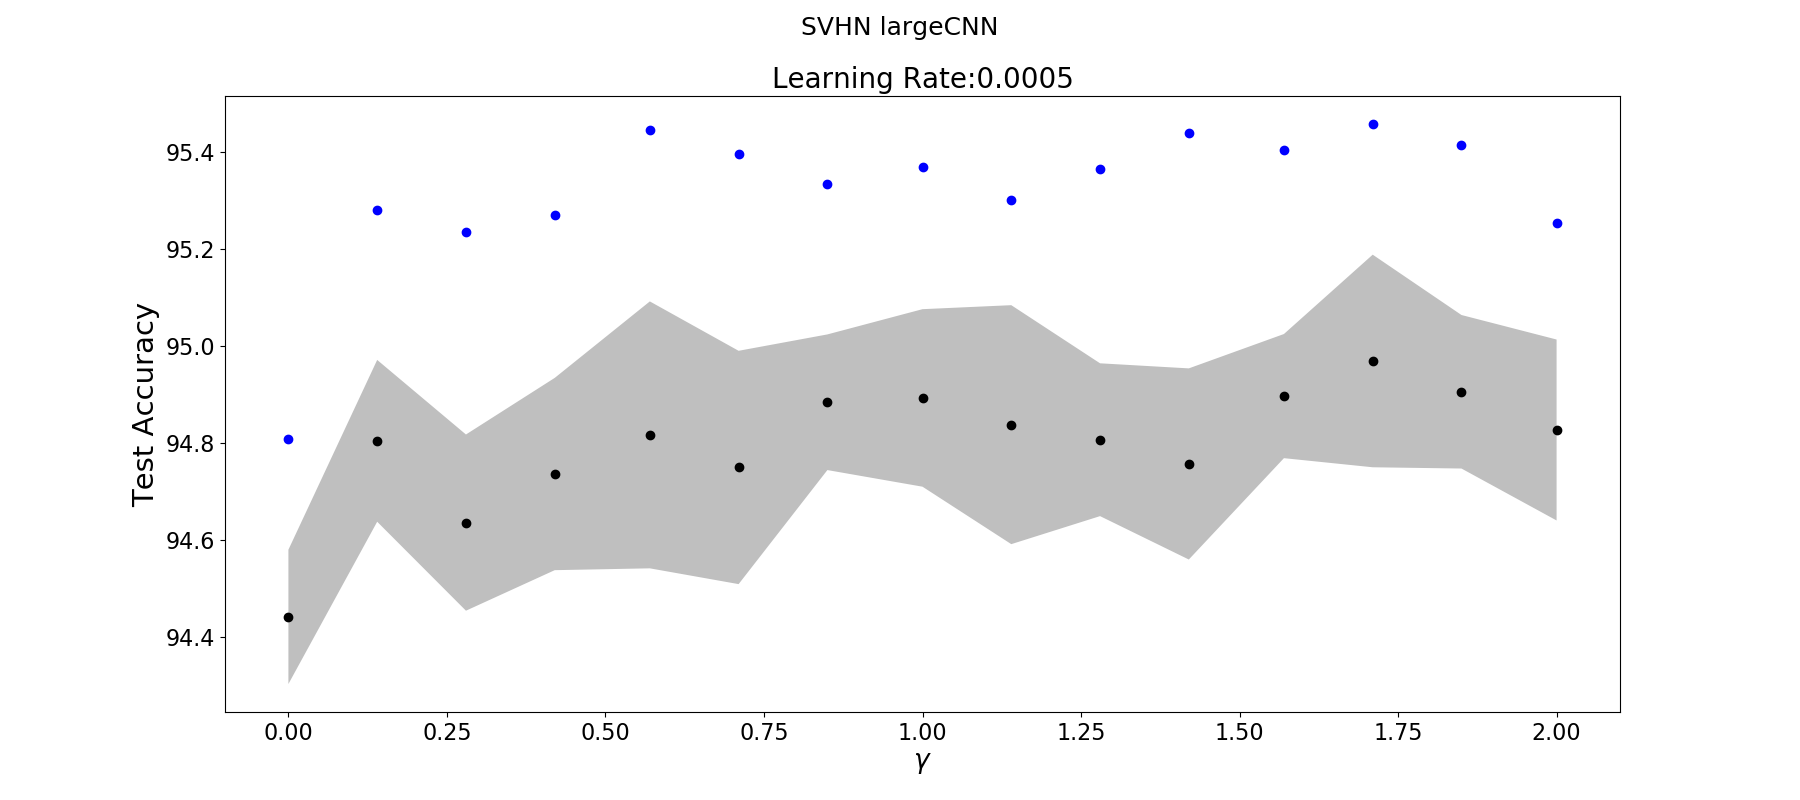}
    \end{figure}
    
\begin{figure}[H]
    \centering
    \includegraphics[width=.99\textwidth]{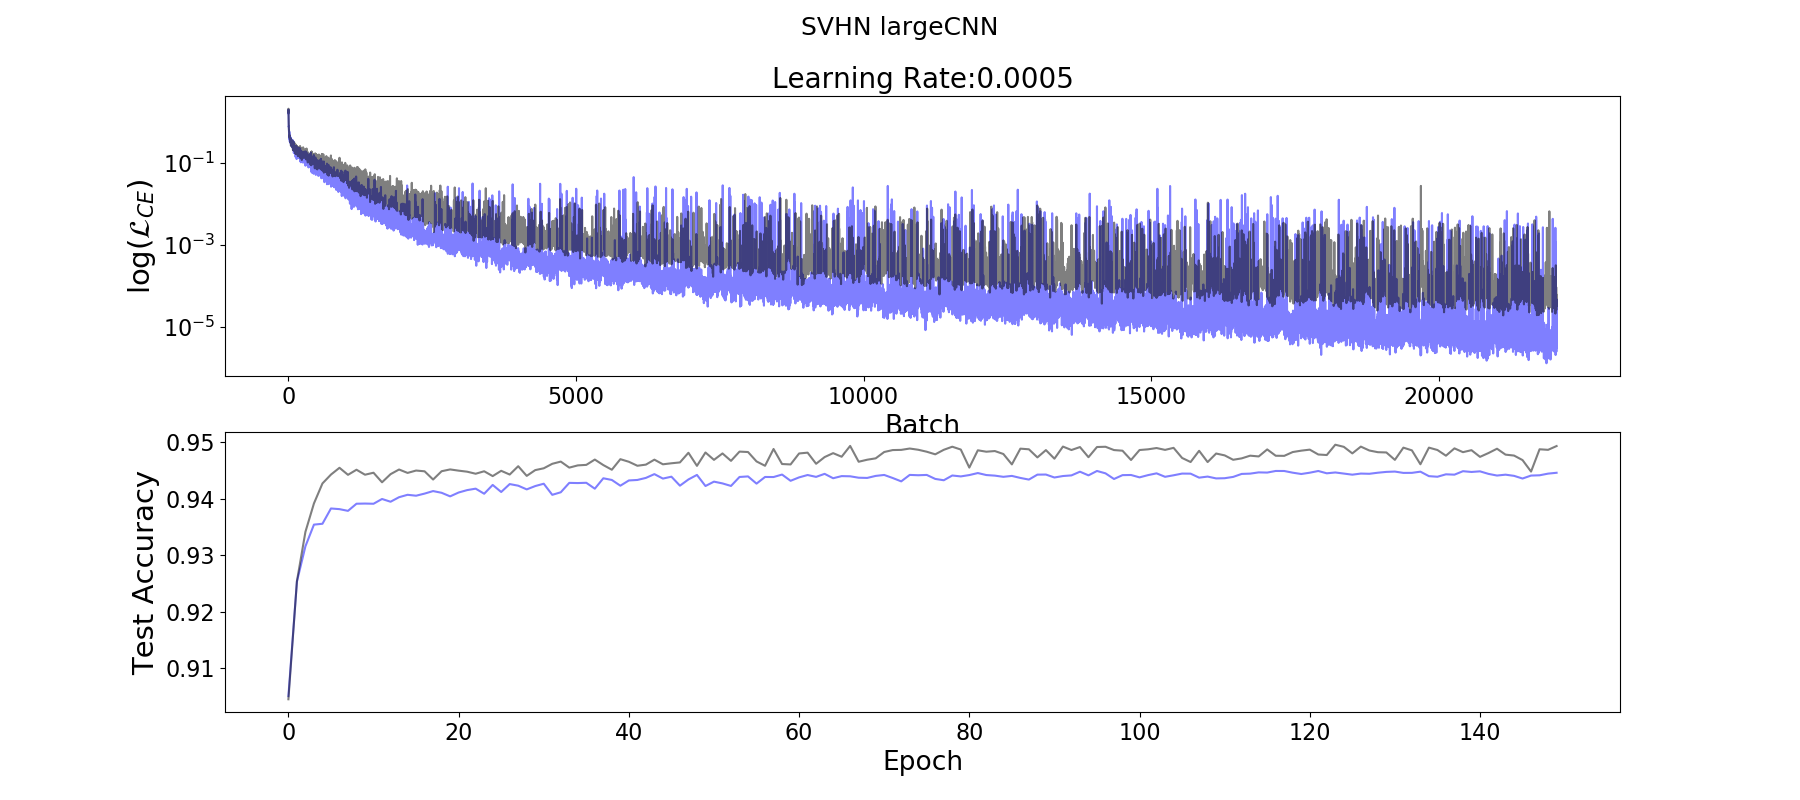}
    \end{figure}
    
      
\begin{figure}[H]
    \centering
    \includegraphics[width=.99\textwidth]{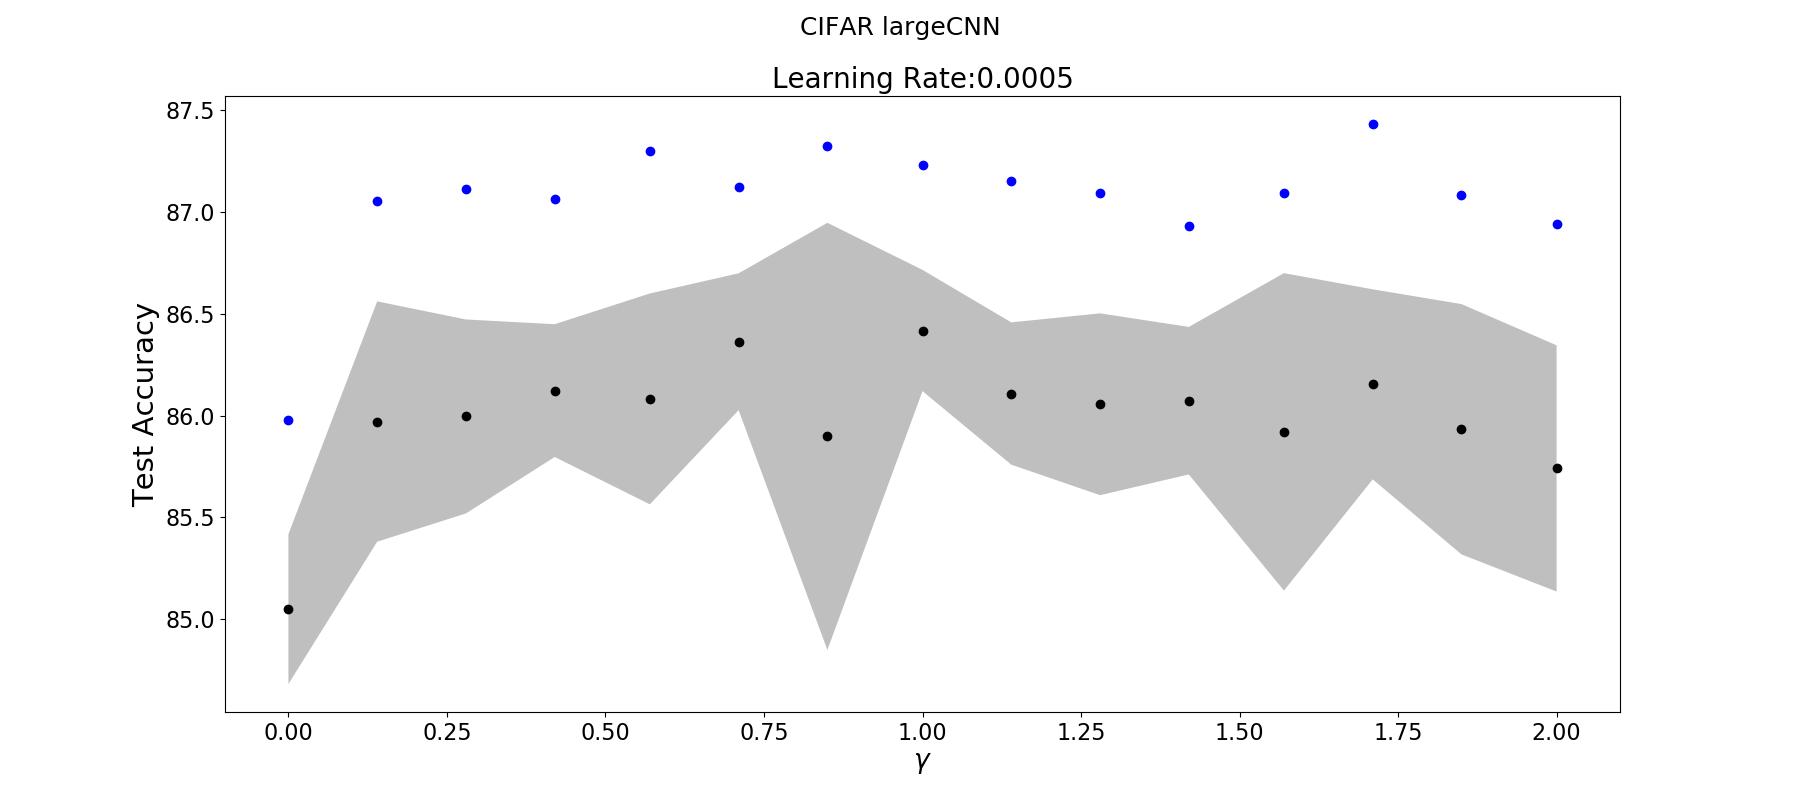}
    \end{figure}
    
\begin{figure}[H]
    \centering
    \includegraphics[width=.99\textwidth]{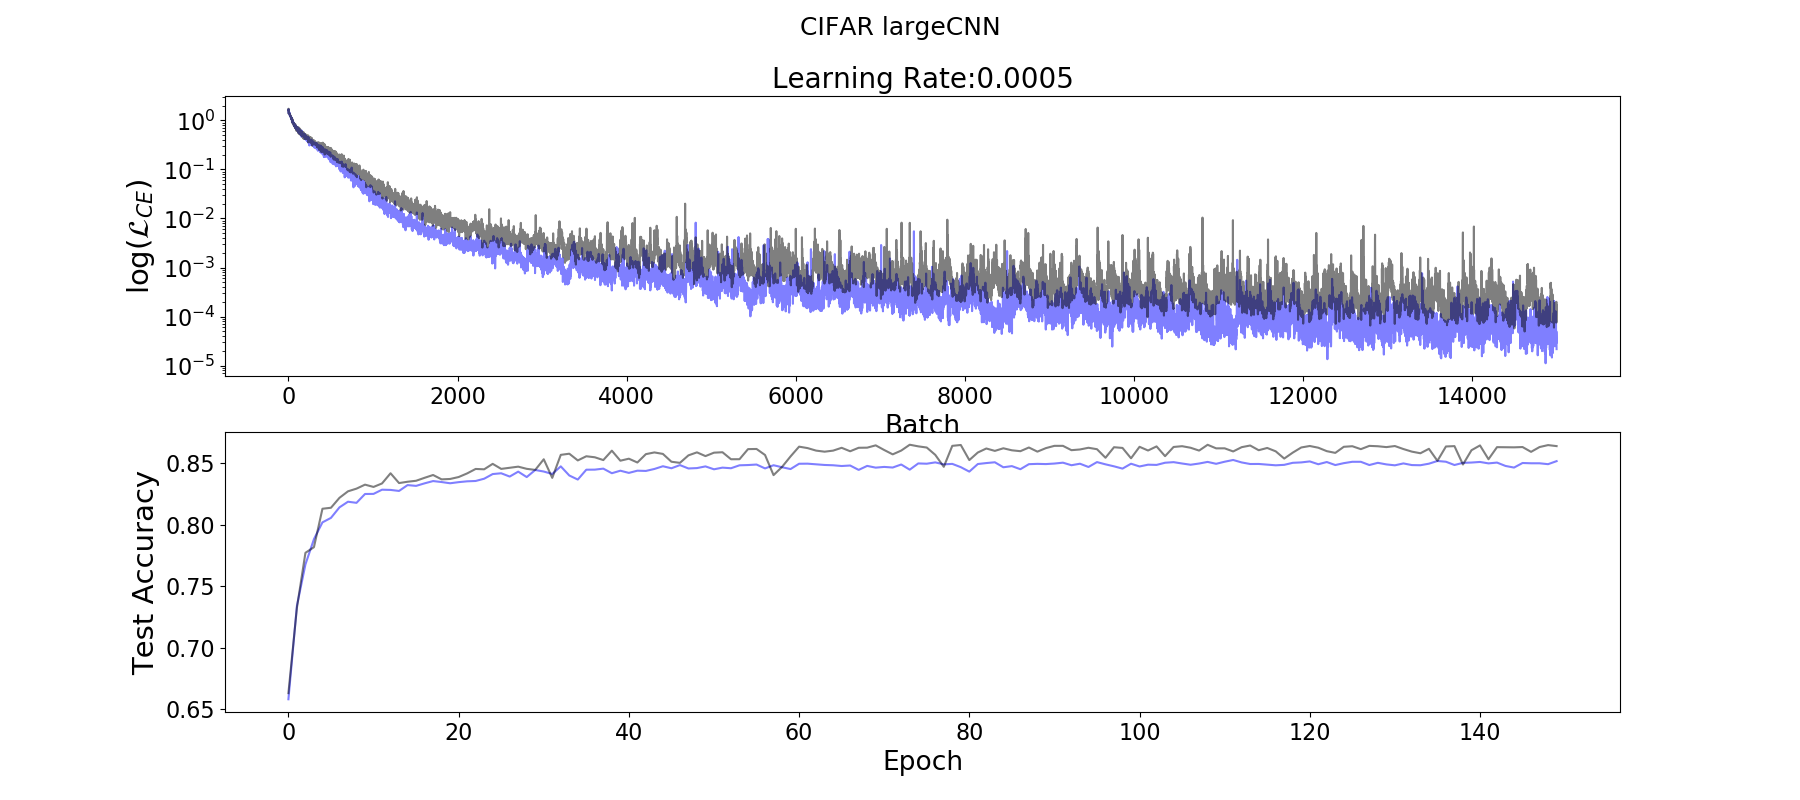}
    \end{figure}
    
      
\begin{figure}[H]
    \centering
    \includegraphics[width=.99\textwidth]{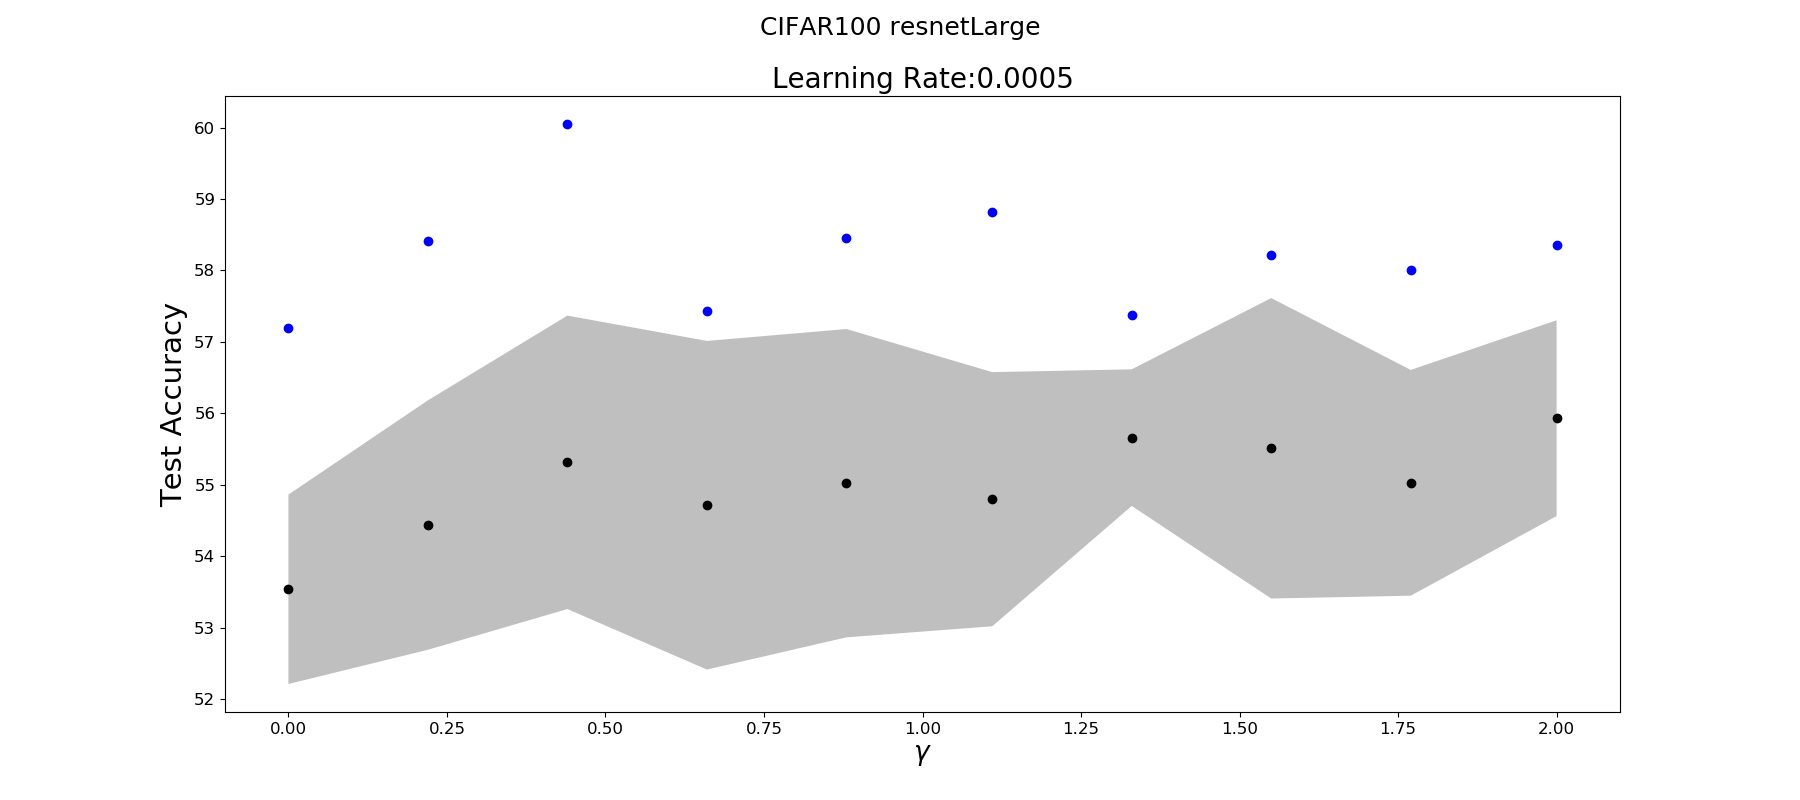}
    \end{figure}
    
\begin{figure}[H]
    \centering
    \includegraphics[width=.99\textwidth]{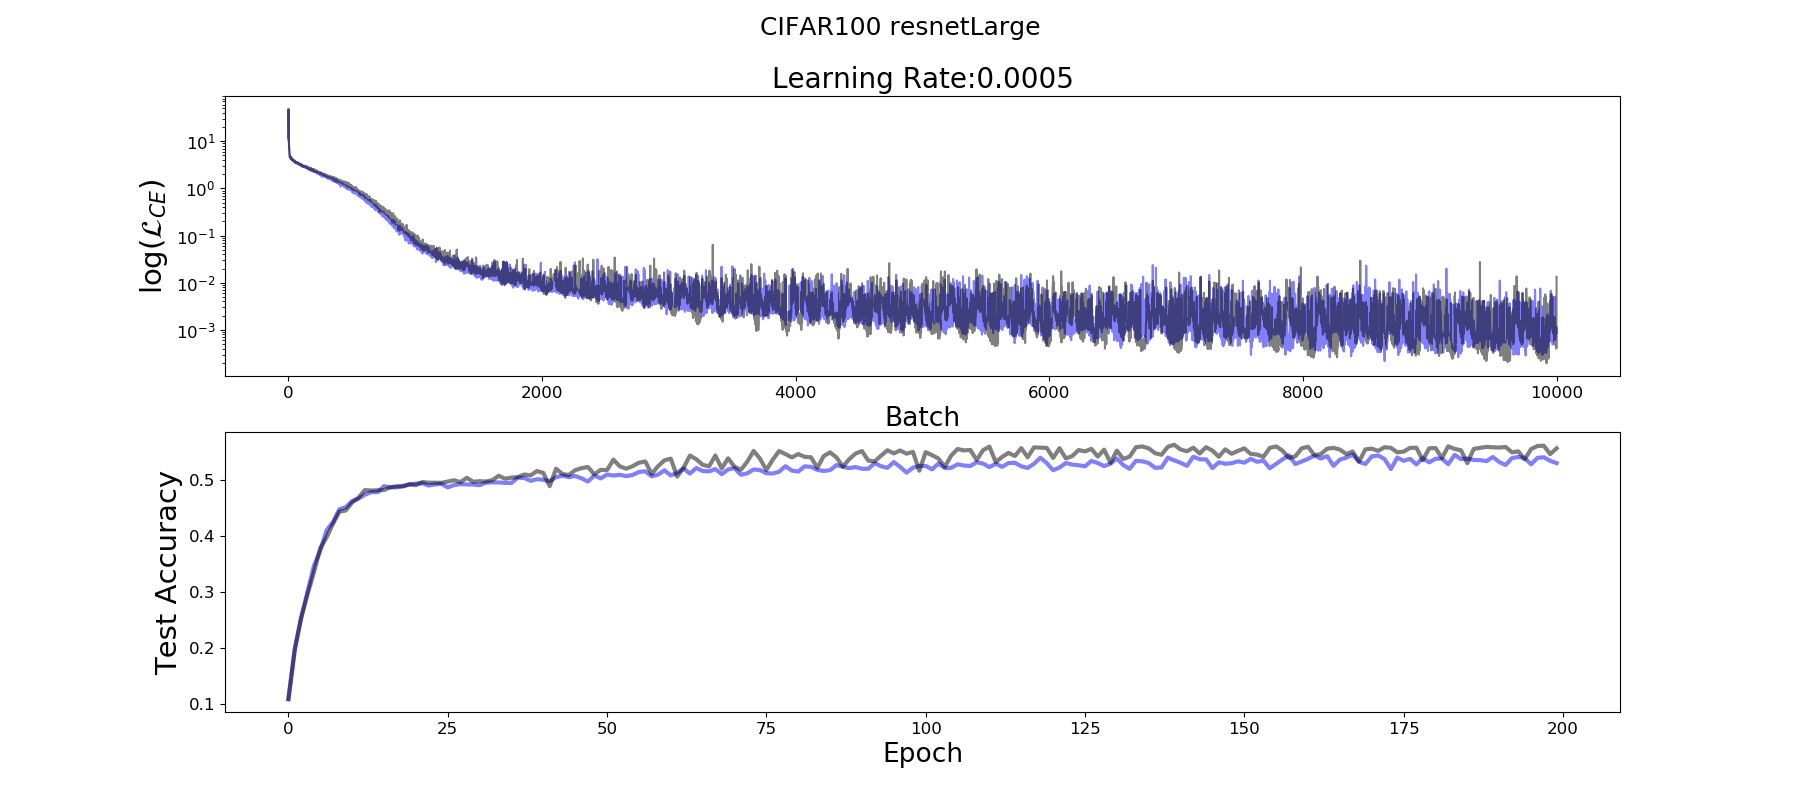}
    \end{figure}
    
