# Supplementary material for: Mad Max: Affine Spline Insights into Deep Learning
Source: arXiv:1805.06576 source file (2018-11-11)
Supplement: Supplementary file 4 [file more_partitioning.tex]

\section{Additional Figures on Partitioning}
\begin{figure}[H]
    \centering
    \includegraphics[width=.99\textwidth]{APPENDIX/MNIST_smallCNNbn0_partitioning18.png}
    \caption{Without batch-normalization and smallCNN}
    \end{figure}
    
    \begin{figure}[H]
    \centering
    \includegraphics[width=.99\textwidth]{APPENDIX/MNIST_smallCNNbn1_partitioning18.png}
    \caption{With batch-normalization and smallCNN}
    \end{figure}
    \begin{figure}[H]
    \centering
    \includegraphics[width=.99\textwidth]{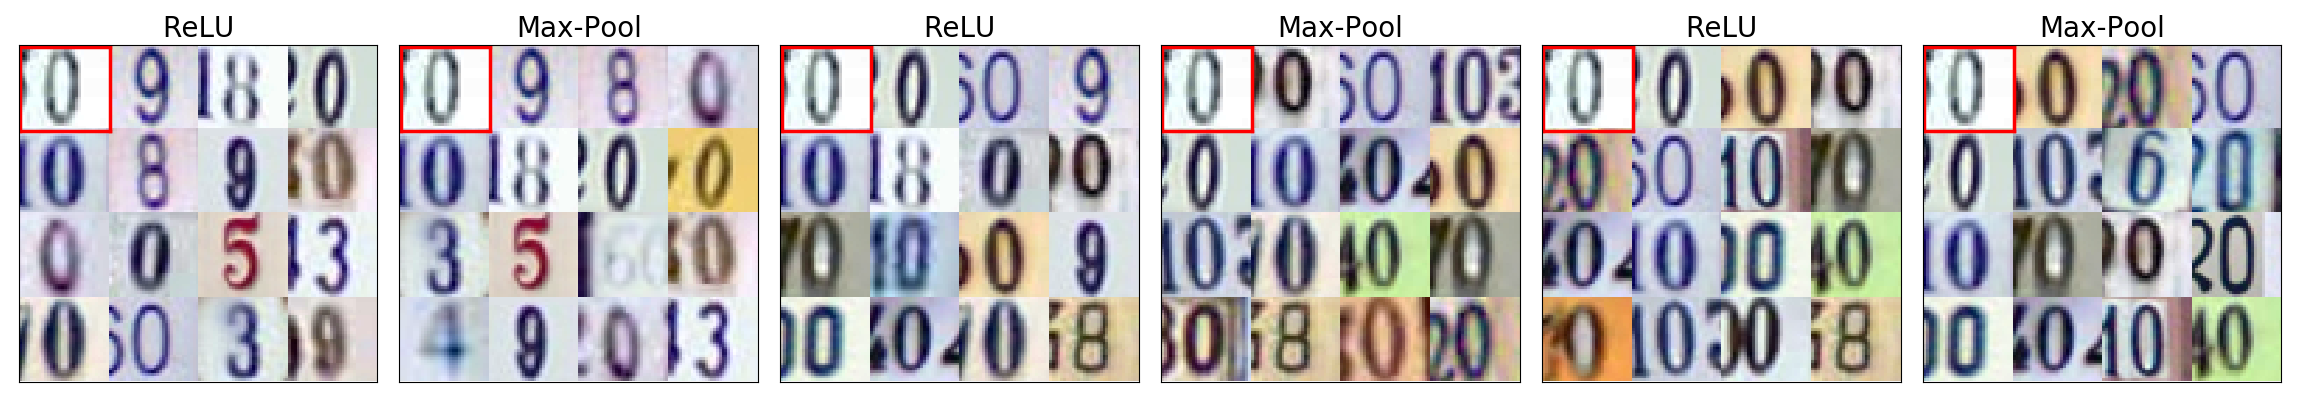}
    \caption{Without batch-normalization and smallCNN}
    \end{figure}
    \begin{figure}[H]
    \centering
    \includegraphics[width=.99\textwidth]{APPENDIX/SVHN_smallCNNbn1_partitioning18.png}
    \caption{With batch-normalization and smallCNN}
    \end{figure}
    
    \begin{figure}[H]
    \centering
    \includegraphics[width=.99\textwidth]{APPENDIX/CIFAR_smallCNNbn0_partitioning18.png}
    \caption{Without batch-normalization and smallCNN}
    \end{figure}
    \begin{figure}[H]
    \centering
    \includegraphics[width=.99\textwidth]{APPENDIX/CIFAR_smallCNNbn1_partitioning18.png}
    \caption{With batch-normalization and smallCNN}
    \end{figure}
    
    
