# Supplementary material for: Mad Max: Affine Spline Insights into Deep Learning
Source: arXiv:1805.06576 source file (2018-11-11)
Supplement: Supplementary file 5 [file more_template.tex]

\section{Additional Template Figures}
\begin{figure}[H]
    \centering
    \includegraphics[width=.99\textwidth]{APPENDIX/CIFAR_smallCNN_l0_Q0_templates1.png}
\end{figure}
\begin{figure}[H]
    \centering
    \includegraphics[width=.99\textwidth]{APPENDIX/CIFAR_smallCNN_l0_Q0_templates2.png}
\end{figure}
\begin{figure}[H]
    \centering
    \includegraphics[width=.99\textwidth]{APPENDIX/CIFAR_smallCNN_l1_Q0_templates1.png}
\end{figure}
\begin{figure}[H]
    \centering
    \includegraphics[width=.99\textwidth]{APPENDIX/CIFAR_smallCNN_l1_Q0_templates2.png}
\end{figure}


\begin{figure}[H]
    \centering
    \includegraphics[width=.99\textwidth]{APPENDIX/CIFAR_largeCNN_l0_Q0_templates1.png}
\end{figure}
\begin{figure}[H]
    \centering
    \includegraphics[width=.99\textwidth]{APPENDIX/CIFAR_largeCNN_l0_Q0_templates2.png}
\end{figure}
\begin{figure}[H]
    \centering
    \includegraphics[width=.99\textwidth]{APPENDIX/CIFAR_largeCNN_l1_Q0_templates1.png}
\end{figure}
\begin{figure}[H]
    \centering
    \includegraphics[width=.99\textwidth]{APPENDIX/CIFAR_largeCNN_l1_Q0_templates2.png}
\end{figure}


\section{Additional Histogram of Template Matching}
\begin{figure}[H]
    \centering
    \includegraphics[width=.99\textwidth]{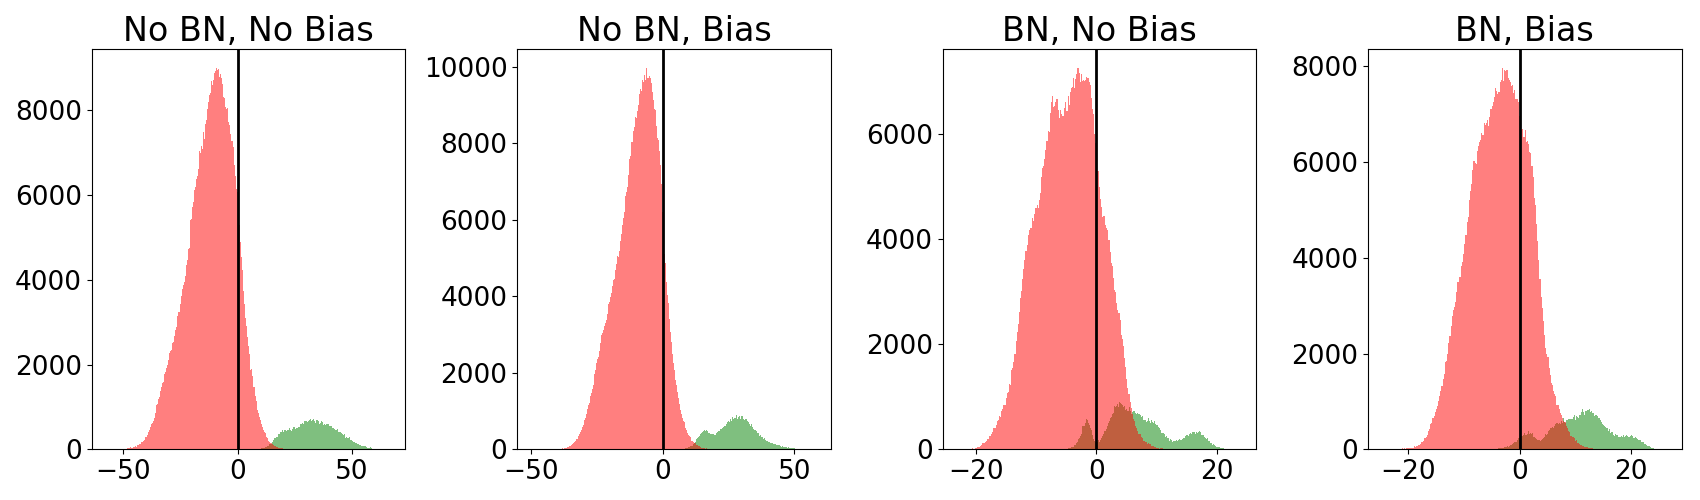}
\end{figure}
\begin{figure}[H]
    \centering
    \includegraphics[width=.99\textwidth]{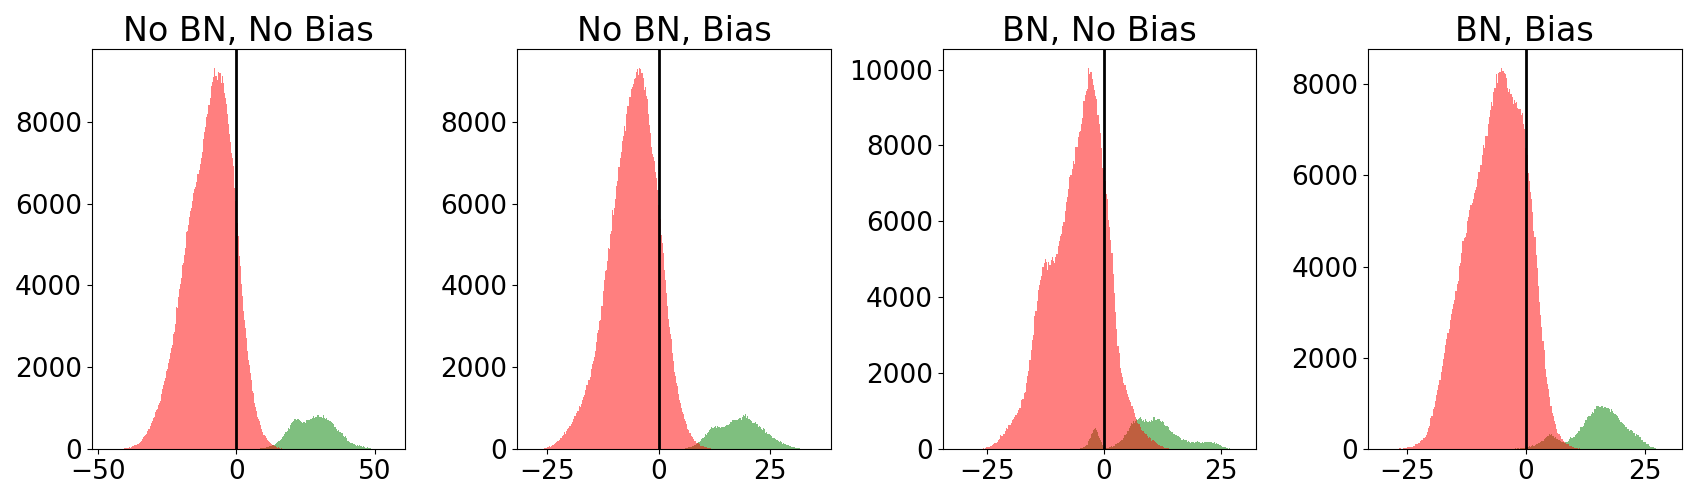}
\end{figure}
\begin{figure}[H]
    \centering
    \includegraphics[width=.99\textwidth]{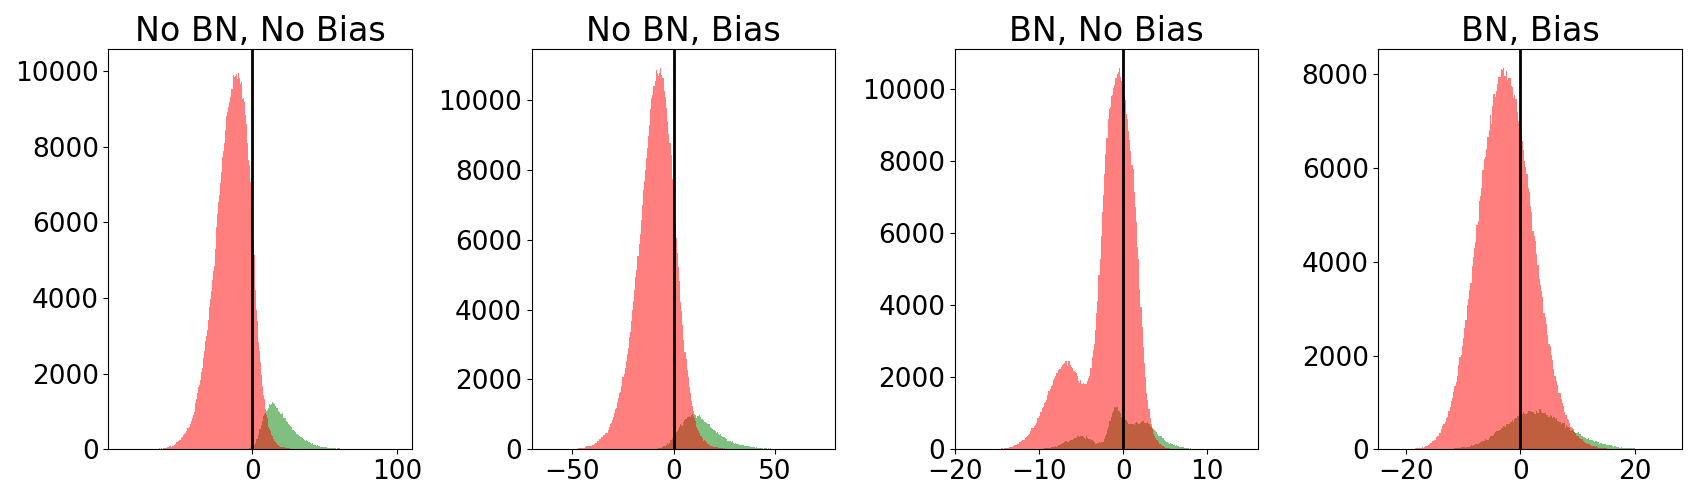}
\end{figure}
\begin{figure}[H]
    \centering
    \includegraphics[width=.99\textwidth]{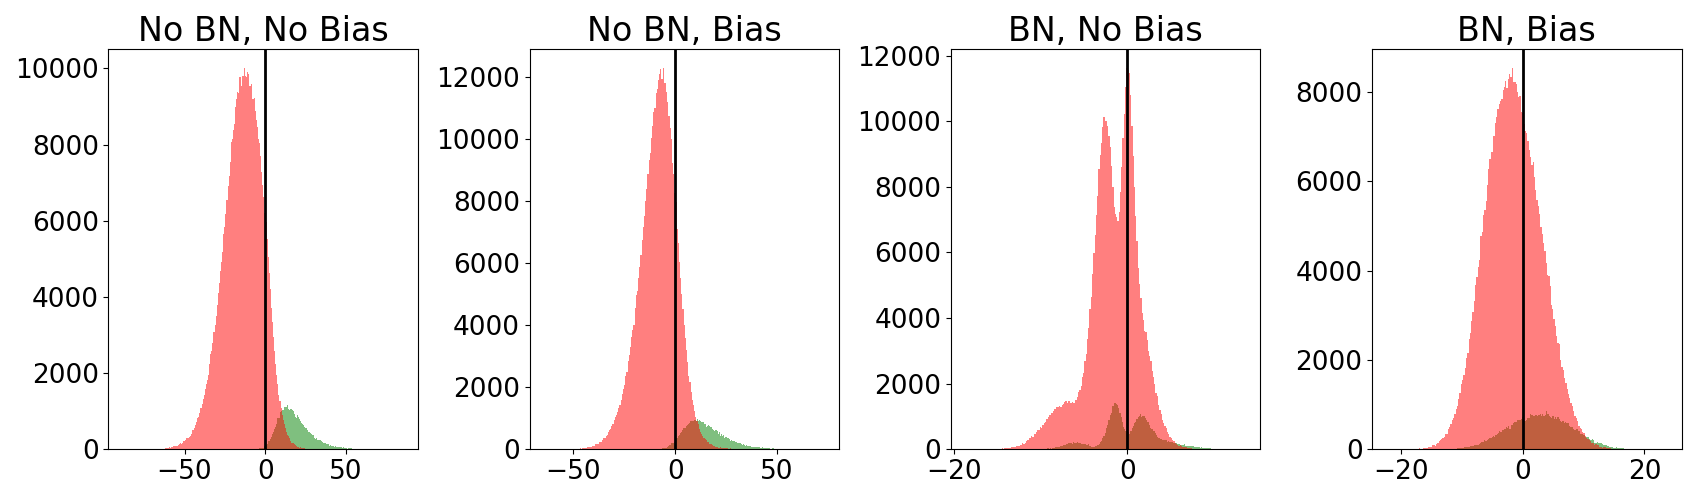}
\end{figure}
